# Supplementary material for: NAG-GS: A Semi-Implicit Stochastic Optimizer with Large-Step Stability
Source: arXiv:2209.14937 source file (2026-10-27)
Supplement: Supplementary file 1 [file appendix-experiments-details.tex]

\section{Additional experimental details}
\label{sec:experiments-details}

In this section we provide additional experimental details.
In particular, we discuss a little bit more our experimental setup and give some insights about NAG-GS as well.

Our computational resources are limited to a single Nvidia DGX-1 with 8 GPUs Nvidia V100.
Almost all experiments were carried out on a single GPU.
The only exception is for the training of ResNet50 on ImageNet which used all 8 GPUs.

\subsection{Fine-Tuning RoBERTa on GLUE}
\label{subsec:details-roberta-glue}

After completion of experiments on toy models, we applied NAG-GS for the training of large neural networks that could be used in practice.
We performed a grid search to come up with an optimal learning rate $\alpha$ for RoBERTa model (see \cref{tab:roberta-glue-grid}).
It is worth mentioning that there is a stability region for NAG-GS which is visible to the naked eye, we highlighted in blue some cells from \cref{tab:roberta-glue-grid} to support this claim.
Furthermore, based on these simple experiments, it appears that choosing $\alpha \sim 10^{-1}$ is a good way to go for a wide variety of tasks.

\begin{table*}[!t]
    \caption{
        Performance in fine-tuning on GLUE benchmark for different learning rate $\alpha$, fixed moment $\mu = 1$, and factor $\gamma \in \{1, 1.5\}$. Largest metric values for NAG-GS optimizer is highlighted with bold typeface. Performance metric is accuracy for all tasks with exception Matthews correlation for \textsc{CoLA} and Pearson correlation for \textsc{STS-B}. Dash in cell means an absence of a run. Higher is better.
    }
    \begin{center}\begin{small}\begin{sc}
        \begin{tabular}{llrrrrrrrrr}
    \toprule
    $\gamma$ & $\alpha$ & \textsc{CoLA} & \textsc{MNLI} & \textsc{MRPC} & \textsc{QNLI} & \textsc{QQP} & \textsc{RTE} & \textsc{SST2} & \textsc{STS-B} & \textsc{WNLI} \\
    \midrule
%    8e+00 & — & — & 68.38 & — & — & 52.71 & 50.92 & 9.84 & \textbf{56.34} \\
%    4e+00 & — & — & 68.38 & — & — & 52.71 & 50.92 & 15.78 & 56.34 \\
%    2e+00 & — & — & 68.38 & — & — & 52.71 & 50.92 & 9.46 & 56.34 \\
%    1e+00 & — & — & 68.38 & — & — & 52.71 & 77.52 & 31.49 & 56.34 \\
%    \cmidrule(lr){1-11}
    1.0 & 8e-01 &                   0.00 & — &                  68.38 &                  50.54 & — & 52.71 & \cellcolor{cyan} 88.42 & 19.86 & \cellcolor{cyan} \textbf{56.34} \\
    {} & 4e-01 &                   0.00 & — & \cellcolor{cyan} 81.13 &                  50.54 & — & 52.71 &                  50.92 & \cellcolor{cyan} 87.36 & \cellcolor{cyan} \textbf{56.34} \\
    {} & 2e-01 & \cellcolor{cyan} 51.16 & — & \cellcolor{cyan} 70.59 & \cellcolor{cyan} 88.93 & — & 52.71 & \cellcolor{cyan} 92.55 & \cellcolor{cyan} 89.34 & \cellcolor{cyan} \textbf{56.34} \\
    {} & 1e-01 & \cellcolor{cyan} \textbf{59.64} & — & \cellcolor{cyan} \textbf{88.73} & \cellcolor{cyan} 90.39 & \cellcolor{cyan} \textbf{91.09} & 52.71 & \cellcolor{cyan} 94.27 & \cellcolor{cyan} 89.97 & \cellcolor{cyan} \textbf{56.34} \\
    \cmidrule(lr){2-11}
    {} & 8e-02 & \cellcolor{cyan} 59.41 & — & \cellcolor{cyan} 86.27 & \cellcolor{cyan} 91.49 & — & \cellcolor{cyan} \textbf{72.56} & \cellcolor{cyan} 93.92 & \cellcolor{cyan} 90.48 & \cellcolor{cyan} \textbf{56.34} \\
     {} & 4e-02 & \cellcolor{cyan} 59.16 & — & \cellcolor{cyan} 87.75 & \cellcolor{cyan} 91.62 & — & \cellcolor{cyan} 72.56 & \cellcolor{cyan} 94.38 & \cellcolor{cyan} \textbf{90.59} & \cellcolor{cyan} \textbf{56.34} \\
     {} & 2e-02 & \cellcolor{cyan} 57.13 & — & \cellcolor{cyan} 88.48 & \cellcolor{cyan} \textbf{91.96} & — & \cellcolor{cyan} 67.87 & \cellcolor{cyan} \textbf{94.72} & \cellcolor{cyan} 90.35 & \cellcolor{cyan} \textbf{56.34} \\
     {} & 1e-02 & \cellcolor{cyan} 53.21 & — & \cellcolor{cyan} 86.52 & \cellcolor{cyan} 91.76 & \cellcolor{cyan} 89.36 & 55.23 & \cellcolor{cyan} 93.92 & \cellcolor{cyan} 88.91 & \cellcolor{cyan} \textbf{56.34} \\
     \cmidrule(lr){2-11}
     {} & 8e-03 & \cellcolor{cyan} 53.94 & — & \cellcolor{cyan} 86.27 &                      — & — & 54.51 & \cellcolor{cyan} 93.58 & \cellcolor{cyan} 89.01 & \cellcolor{cyan} \textbf{56.34} \\
     {} & 4e-03 & \cellcolor{cyan} 49.25 & — & \cellcolor{cyan} 78.92 &                      — & — & 53.07 & \cellcolor{cyan} 93.69 & \cellcolor{cyan} 86.38 & \cellcolor{cyan} \textbf{56.34} \\
     {} & 2e-03 & \cellcolor{cyan} 40.73 & — &                  68.38 &                      — & — & 52.71 & \cellcolor{cyan} 93.35 & \cellcolor{cyan} 79.56 & \cellcolor{cyan} \textbf{56.34} \\
     {} & 1e-03 &                   0.00 & — &                  68.38 & \cellcolor{cyan} 86.88 & \cellcolor{cyan} 86.01 & 52.71 & \cellcolor{cyan} 93.35 & 58.97 & 43.66 \\
%    \cmidrule(lr){1-11}
%    8.0e-04 & 0.00 & — & — & 68.38 & — & — & 52.71 & \cellcolor{cyan} 92.55 & 38.33 & 43.66 \\
%    4.0e-04 & 0.00 & — & — & 68.38 & — & — & 52.71 & \cellcolor{cyan} 91.63 & 0.80 & 43.66 \\
%    2.0e-04 & 0.00 & — & — & 68.38 & — & — & 47.29 & \cellcolor{cyan} 87.73 & -6.78 & 43.66 \\
%    1.0e-04 & 0.00 & — & — & 68.38 & 57.37 & 80.32 & 47.29 & 50.92 & -10.39 & 43.66 \\
%    \cmidrule(lr){1-11}
%    8.0e-05 & 0.00 & — & — & 68.38 & — & — & 47.29 & 50.92 & -11.16 & 43.66 \\
%    4.0e-05 & 0.00 & — & — & 68.38 & — & — & 47.29 & 50.92 & -11.56 & 43.66 \\
%    2.0e-05 & 0.00 & — & — & 68.38 & — & — & 47.29 & 50.92 & -11.56 & 43.66 \\
%    1.0e-05 & 0.00 & — & — & 68.38 & — & — & 47.29 & 50.92 & -11.55 & 43.66 \\
%    \cmidrule(lr){1-11}
%    8.0e-06 & 0.00 & — & — & 68.38 & — & — & 47.29 & 50.92 & -11.55 & 43.66 \\
%    4.0e-06 & 0.00 & — & — & 68.38 & — & — & 47.29 & 50.92 & -11.55 & 43.66 \\
%    2.0e-06 & 0.00 & — & — & 68.38 & — & — & 47.29 & 50.92 & -11.55 & 43.66 \\
%    1.0e-06 & 0.00 & — & — & 68.38 & — & — & 47.29 & 50.92 & -11.55 & 43.66 \\
    \midrule
    1.5 & 8e-01 &  0.00 & 35.45 & 68.38 & 50.54 & 89.33 & 52.71 & 91.17 & 24.84 & \textbf{56.34} \\
     {} & 4e-01 &  0.00 & 80.29 & 68.38 & 50.54 & 90.23 & 52.71 & 91.86 & 88.62 & \textbf{56.34} \\
     {} & 2e-01 &  0.00 & 82.01 & 84.80 & 90.04 & 91.01 & 52.71 & 93.46 & 89.44 & \textbf{56.34} \\
     {} & 1e-01 & \textbf{61.48} & 86.94 & 87.75 & 50.54 & 90.91 & 72.56 & 94.38 & 90.07 & \textbf{56.34} \\
    \cmidrule(lr){2-11}
     {} & 8e-02 & 57.77 & 87.06 & 86.76 & 90.92 & \textbf{90.92} & \textbf{73.65} & 94.27 & \textbf{90.21} & \textbf{56.34} \\
     {} & 4e-02 & 59.97 & \textbf{87.24} & \textbf{89.71} & \textbf{92.42} & 90.59 & 70.04 & \textbf{94.50} & 90.11 & \textbf{56.34} \\
     {} & 2e-02 & 56.50 & 87.25 & 87.75 & 91.65 & 89.89 & 61.73 & 94.15 & 90.03 & \textbf{56.34} \\
     {} & 1e-02 & 55.08 & 86.72 & 85.29 & 91.62 & 88.91 & 55.23 & 93.69 & 88.91 & \textbf{56.34} \\
    \cmidrule(lr){2-11}
     {} & 8e-03 & 50.79 & 86.46 & 83.58 & 90.99 & 88.92 & 56.68 & 93.35 & 87.92 & \textbf{56.34} \\
     {} & 4e-03 & 48.74 & 85.51 & 72.30 & 90.46 & 87.87 & 52.71 & 93.23 & 84.79 & \textbf{56.34} \\
     {} & 2e-03 &  0.00 & 84.64 & 68.38 & 87.94 & 86.80 & 52.71 & 93.46 & 78.15 & 43.66 \\
     {} & 1e-03 &  0.00 & 83.06 & 68.38 & 86.66 & 85.38 & 52.71 & 92.78 & 34.77 & 43.66 \\
    \bottomrule
\end{tabular}

    \end{sc}\end{small}\end{center}
    \label{tab:roberta-glue-grid}
\end{table*}

In the subsequent experiments we limited ourselves to RoBERTa's training on small GLUE tasks in order to study relations between $\alpha$ and $\gamma$ in the context of high-dimensional non-convex objective functions (see \cref{fig:hyperopt-mrpc}).
One can see that there is oblong area in which NAG-GS converges pretty well.
The ridge of this area can be empirically described with linear equation $\log~\alpha = a \log~\gamma + b$ in logarithmic domain.
%Later, we get back to experiments of such kind but for other type of model (see \cref{subsec:phase-diagrams}).
In \cref{subsec:phase-diagrams}, we perform similar study for other types of model.

\begin{figure}[!t]
    \centering
    \begin{subfigure}{0.49\textwidth}
        \includegraphics[width=\textwidth]{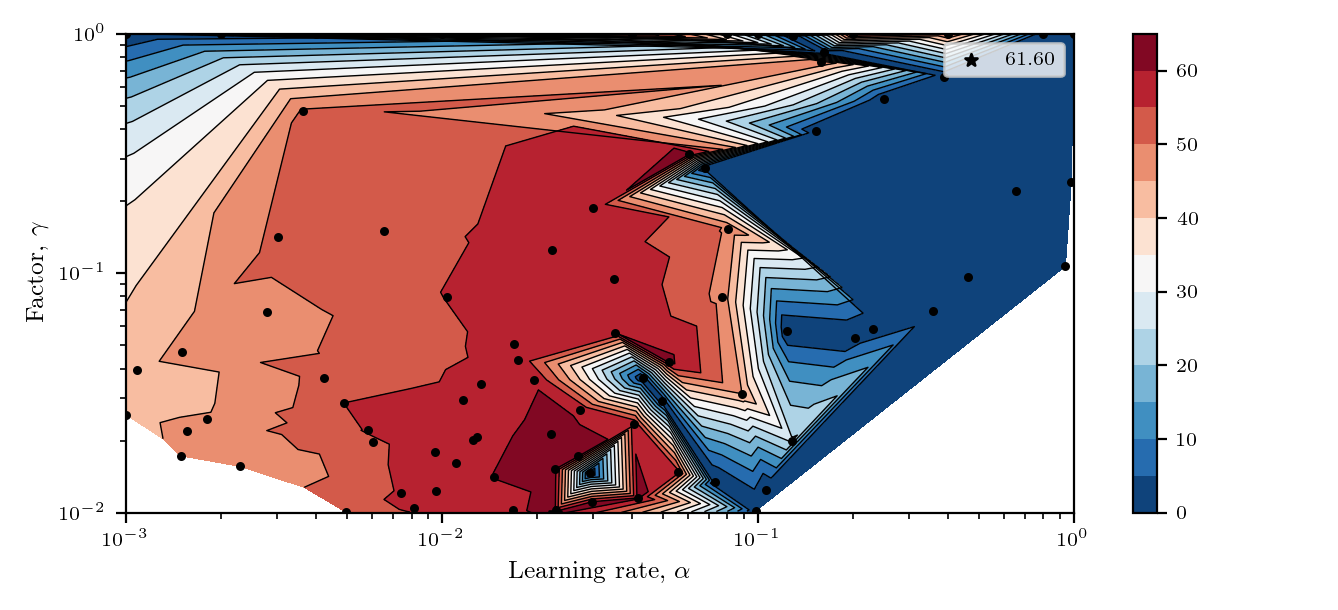}
    \end{subfigure}
    \hfill
    \begin{subfigure}{0.49\textwidth}
        \includegraphics[width=\textwidth]{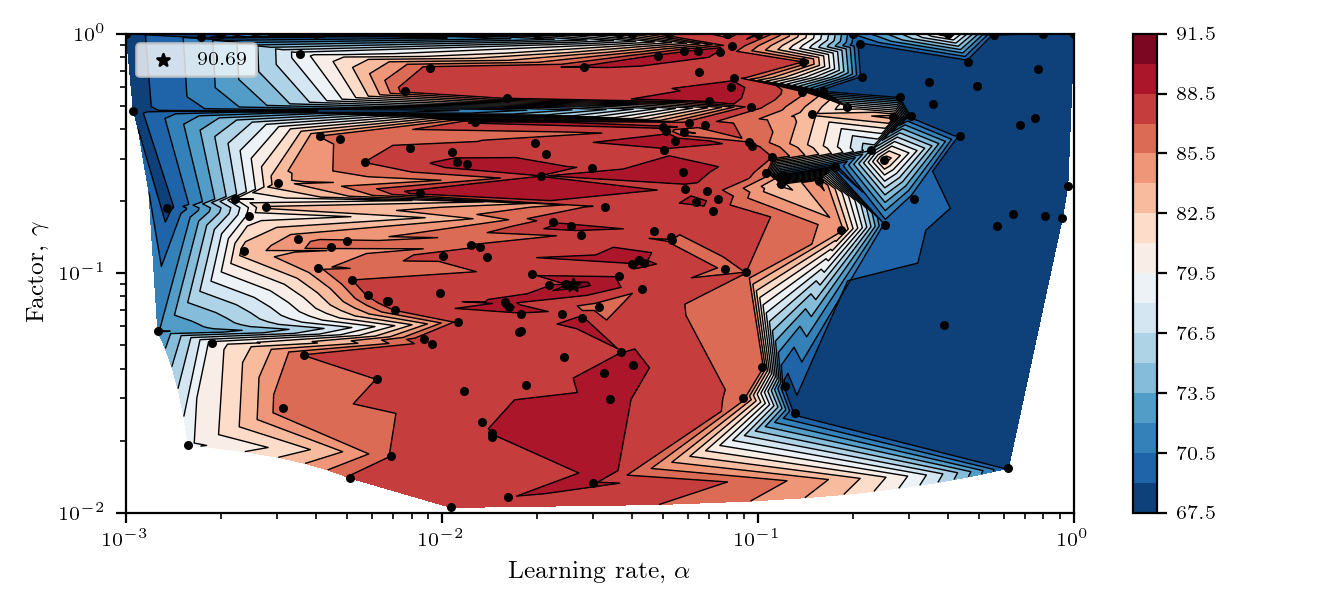}
    \end{subfigure}
    \caption{
        Landscape of accuracy metric of RoBERTa model fine-tuned on \textsc{CoLA} (top) \textsc{MRPC} (bottom) with NAG-GS. Hyperparameter optimization algorithms samples learning rate $\alpha$ from $[10^{-3},\,10^0]$ and factor $\gamma$ from $[10^{-2},\,10^0]$. Both hyperparameters are sampled from log-uniform distribution. Symbol $\star$ marks the best points.
    }
    \label{fig:hyperopt-mrpc}
\end{figure}

\subsection{Phase diagrams}
\label{subsec:phase-diagrams}

In~\cref{subsec:hessian-spectrum} we mentioned that the lowest eigenvalues $\mu$ of approximated Hessian matrices evaluated during the training of ResNet20 model were negative.
Furthermore, our theoretical analysis of NAG-GS in the convex case include some conditions on the optimizer parameters $\alpha$, $\gamma$, and $\mu$. In particular it is required that $\mu > 0$ and $\gamma \ge \mu$.
In order to bring some insights about these remarks in the non-convex setting and inspired by \cite{velikanov2022view}, we experimentally study the convergence regions of NAG-GS and sketch out the phase diagrams of convergence for different projection planes, see~\cref{fig:contour-gamma-mu}.

\begin{figure}[!t]
    \centering
    \includegraphics{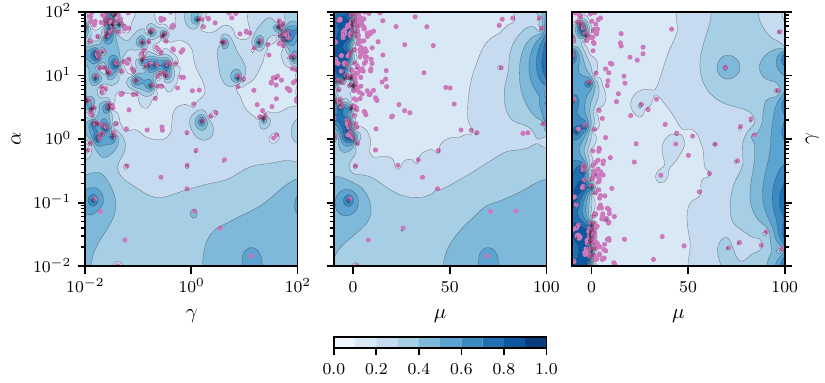}
    \caption{
        Landscapes of classification error for ResNet-20 model trained on \textsc{CIFAR-10} with NAG-GS after projections onto $\alpha-\gamma$, $\alpha-\mu$ and $\gamma - \mu$ planes (from left to right).
        Hyperparameter optimization algorithm samples learning rate $\alpha$ from $[10^{-2},\,10^2]$, factor $\gamma$ from $[10^{-2},\,10^2]$, and factor $\mu$ from $[-10, 90]$. Hyperparameters $\alpha$ and $\gamma$ are sampled from log-uniform distribution, hyperparameter $\mu$ are sampled from uniform distribution.
    }
    \label{fig:contour-gamma-mu}
\end{figure}

We consider the same setup as in~\cref{par:resnet20} and use hyperoptimization library \textsc{Optuna}~\cite{akiba2019optuna}.
Our preliminary experiments on RoBERTa (see~\cref{subsec:details-roberta-glue}) shows that $\alpha$ should be of magnitude $10^{-1}$.
With the estimate of Hessian spectrum of ResNet20 we define the following search space
\[
    \alpha \sim \mathrm{LogUniform}(10^{-2}, 10^2), \quad
    \gamma \sim \mathrm{LogUniform}(10^{-2}, 10^2), \quad
    \mu \sim \mathrm{Uniform}(-10, 100).
\]
We sample a fixed number of triples and train ResNet20 model on CIFAR-10.
Objective function is a top-1 classification error.

We report that there is a convergence almost everywhere within the projected search space onto $\alpha$-$\gamma$ plane~(see \cref{fig:contour-gamma-mu}).
The analysis of projections onto $\alpha$-$\mu$ and $\gamma$-$\mu$ planes brings different conclusions: there are regions of convergence for negative $\mu$ for some $\alpha < \alpha_{th}$ and $\gamma > \gamma_{th}$.
Also, as it was mentioned in, there is a subdomain of negative $\mu$ comparable to a domain of positive $\mu$ in a sense of the target metrics.
Moreover, the majority of sampled points are located in the vicinity of the band $\lambda_{min} < \mu < \lambda_{max}$.

\subsection{Implementation Details}
\label{subsec:implementation-details}

In our work we implemented NAG-GS in PyTorch \cite{pytorch2017automatic} and JAX \cite{jax2018github,deepmind2020jax}.
Both implementations are used in our experiments and available online\footnote{\url{https://github.com/user/nag-gs}}.
According to \cref{alg:nag_gsgeneral} the size of NAG-GS state equals to number of optimization parameters which makes NAG-GS comparable to SGD with momentum.
It worth to note that Adam-like optimizers has twice larger state than NAG-GS.
Arithmetic complexity of NAG-GS is linear $O(n)$ in the number of parameters.
\cref{tab:benchmark} shows a comparison of computational efficiency of common optimizers used in practice.
Although forward pass and gradient computations usually give the main contribution to training step, there is a settings when efficiency of gradient updates are important (e.g. batch size or a number of intermediate activations are small with respect to a number of parameters).

\begin{table*}[!t]
    \caption{
        The comparision of a single step duration for different optimizers on \textsc{ResNet20} on \textsc{CIFAR-10}. \textsc{Adam}-like optimizers have in twice larger state than momentum \textsc{SGD}s or \textsc{NAG-GS}.
    }
    \begin{center}\begin{small}\begin{sc}
        \input{tbl/benchmark.tex}
    \end{sc}\end{small}\end{center}
    \label{tab:benchmark}
\end{table*}
